# Supplementary material for: Robust causal structure learning with some hidden variables
Source: arXiv:1708.01151 ancillary file (2018-08-04)
Supplement: Supplementary file 1 [file Appendix.pdf]

# Appendix to "Learning Directed Acyclic Graphs with Hidden Variables via Latent Gaussian Graphical Model Selection"

August 3, 2017

# A Proof of Theorem 3.1

Throughout, we make use of a number matrix norms that we define here. For any matrix $M$, we let $||M||_2$ be the spectral norm of $M$, *i.e.* $M$'s largest singular value. $||M||_\infty$ is the largest entry of $M$ in magnitude, *i.e.* $||M||_\infty = \max_{i,j} |M_{ij}|$. $||M||_1$ is defined as the entrywise $\ell_1$-norm: $||M||_1 = \sum_{i,j} |M_{ij}|$. $|||M|||_1$ is defined to be the maximum absolute column sum of $M$, *i.e.* $|||M|||_1 = \max_j \sum_i |M_{ij}|$. Likewise, $|||M|||_\infty$ is the maximum absolute *row* sum of $M$, *i.e.* $|||M|||_\infty = \max_i \sum_j |M_{ij}|$. Moreover, we let $\text{sign}(M)$ denote the matrix which assigns each coefficient to its sign: $(\text{sign}(M))_{ij} = \text{sign}(M_{ij})$.

We recall here the main consequences of assumption (A1), which entails the consistency of the LRpS estimator of Chandrasekaran et al. [2012]. Describing (A1) in detail requires numerous definitions and would take us beyond the scope of this paper. We therefore refer the reader to Chandrasekaran et al. [2012] for more details and limit ourselves to the results that are used in our proof. In particular, we recall from the main paper that (A1) assumes $\gamma \in [\frac{3\xi(T)}{C}, \frac{C}{2\mu(\Omega)}]$, with $C$ a constant which depends on the Fisher information matrix only.

**Theorem A.1.** *(Theorem 4.1 of Chandrasekaran et al. [2012])*
*Under assumption (A1), we have with probability greater than* $1 - 2\exp(-p)$

- $\frac{1}{\gamma}||\hat{K}_{nO} - K^*_{nO}||_\infty \leq C_1 \frac{1}{\xi(T)}\sqrt{\frac{p}{n}}$,
- $\text{sign}(\hat{K}_{nO}) = \text{sign}(K^*_{nO})$,
- $\text{rank}(\hat{L}_n) = \text{rank}(L^*_n)$,

*where* $C_1$ *is a constant which depends on the Fisher information matrix only.*

Recalling that the matrix $K^*_{nO}$ is sparse with degree $q'_n$, this allows us to derive a useful result about the spectral norm of the error terms.

**Corollary A.1.** *Assume that assumption (A1), (A2) and (A3) hold. Then, for any* $\delta \in (0,1)$*, there exists* $n_0 \in \mathbb{N}$ *such that for all* $n \geq n_0$

$$\mathbb{P}(||\hat{K}_{nO} - K^*_{nO}||_2 > \delta,\ \{\text{sign}(\hat{K}_{nO}) = \text{sign}(K^*_{nO})\}) \leq C_2 \exp(-C_3 n q_n'^{-2} \delta^2),$$

*where* $C_3$ *is a strictly positive constant which depends on the Fisher information matrix only, and* $C_2$ *is a strictly positive constant.*

*Proof.* By (A1), $\frac{1}{\gamma} \in [\frac{2\mu(\Omega)}{C}, \frac{C}{3\xi(T)}]$, so that

$$\frac{1}{\gamma}||\hat{K}_{nO} - K^*_{nO}||_\infty \leq \frac{C}{3\xi(T)}||K^*_{nO} - \hat{K}_{nO}||_\infty.$$

Thus, by Theorem A.1

$$||\hat{K}_{nO} - K^*_{nO}||_\infty \leq \frac{3C_1}{C}\sqrt{\frac{p_n}{n}}$$

hold with probability greater than $1 - 2\exp(-p_n)$. This implies

$$\mathbb{P}\left(||\hat{K}_{nO} - K^*_{nO}||_\infty > \frac{3C_1}{C}\sqrt{\frac{p_n}{n}},\ \{\text{sign}(\hat{K}_{nO}) = \text{sign}(K^*_{nO})\}\right) \leq 2\exp(-p_n). \qquad (1)$$

Now, remark that $\text{sign}(\hat{K}_{nO}) = \text{sign}(K^*_{nO})$ entails that the matrix $K^*_{nO}$ and $\hat{K}_{nO}$ have the same non-zero pattern. However, while their non-zero entries have the same locations, they do not necessarily have the same values. Therefore,

$$(\text{sign}(\hat{K}_{nO}) = \text{sign}(K^*_{nO})) \Rightarrow (\text{degree}(\hat{K}_{nO} - K^*_{nO}) \leq q_n').$$

Now, by Hölder's inequality we obtain

$$||\hat{K}_{nO} - K^*_{nO}||_2 \leq \sqrt{|||\hat{K}_{nO} - K^*_{nO}|||_1 |||\hat{K}_{nO} - K^*_{nO}|||_\infty}$$

which simplifies to

$$||\hat{K}_{nO} - K^*_{nO}||_2 \leq |||\hat{K}_{nO} - K^*_{nO}|||_\infty,$$

since $\hat{K}_{nO} - K^*_{nO}$ is symmetric. From the definition of $|||\cdot|||_\infty$ and the fact that degree$(\hat{K}_{nO} - K^*_{nO}) \leq q'_n$, we conclude that $||\hat{K}_{nO} - K^*_{nO}||_2 \leq q'_n ||\hat{K}_{nO} - K^*_{nO}||_\infty$ on the set $\{\text{sign}(\hat{K}_{nO}) = \text{sign}(K^*_{nO})\}$.

Using this result in conjunction with (1), we have

$$\mathbb{P}\left(||\hat{K}_{nO} - K^*_{nO}||_2 > \frac{3C_1 q'_n}{C}\sqrt{\frac{p_n}{n}},\ \{\text{sign}(\hat{K}_{nO}) = \text{sign}(K^*_{nO})\}\right) \leq C_2 \exp(-p_n),$$

where we set $C_2 = 2$.

Finally, by assumptions (A2) and (A3), we know that $q'_n \sqrt{p_n} = o(\sqrt{n})$, so that for any $\delta \in (0,1)$, there exists an $n_0$ such that for $n \geq n_0$ we have $\frac{3C_1 q'_n}{C}\sqrt{\frac{p_n}{n}} \leq \delta$. Thus, for $n$ large enough, we have

$$\mathbb{P}\left(||\hat{K}_{nO} - K^*_{nO}||_2 > \delta,\ \{\text{sign}(\hat{K}_{nO}) = \text{sign}(K^*_{nO})\}\right) \leq C_2 \exp(-C_3 n {q'}_n^{-2} \delta^2),$$

for any $\delta \in (0,1)$. □

In what follows, we derive a couple of lemmas which are similar to Lemma 5 and 7 of Harris and Drton [2013] but differ from them in that they are expressed in terms of the spectral norm ($||\cdot||_2$), as opposed to the max norm ($||\cdot||_\infty$).

**Lemma A.1.** *Suppose $A \in \mathbb{R}^{r\times r}$ is a positive definite matrix with minimal eigenvalue $\lambda_{\min}(A)$. If $E \in \mathbb{R}^{r\times r}$ is a matrix which satisfies $||E||_2 \leq \epsilon \leq \lambda_{\min}(A)/2$, then $A + E$ is invertible and*

$$||(A+E)^{-1} - A^{-1}||_2 \leq \frac{2\epsilon}{\lambda^2_{\min}(A)}.$$

*Proof.* By definition, we know that $||A^{-1}||_2 = \frac{1}{\lambda_{\min}(A)}$. Thus, by our assumption on $||E||_2$ and the submultiplicity of the spectral norm, we have

$$||EA^{-1}||_2 \leq ||E||_2 ||A^{-1}||_2 \leq \frac{\epsilon}{\lambda_{\min}(A)} < 1.$$

Now, writing $UDU^{-1}$ for the eigendecomposition of $A^{-1}E$, we have

$$A + E = A(I_r + A^{-1}E) = AU(I_r + D)U^{-1}.$$

Since $||A^{-1}E||_2 < 1$, we know that for all $i \in \{1, \dots, r\}$, $|D_{ii}| < 1$ and therefore $(I_r + D)_{ii} > 0$. This proves our claim about $(A + E)$ being invertible.

For the second part, we follow the arguments of Lemma 5 of Harris and Drton [2013] where the proof of a similar claim is given. More precisely, a bound on $||(A+E)^{-1} - A^{-1}||_\infty$ is derived under some assumptions about $||E||_\infty$.

In the proof of Lemma 5 of Harris and Drton [2013], it is shown that $||EA^{-1}||_2 \leq \frac{\epsilon}{\lambda_{\min}(A)}$, for $\epsilon < \lambda_{\min}(A)$, entails

$$||(A + E)^{-1} - A^{-1}||_2 \leq \frac{\epsilon}{\lambda_{\min}(A)(\lambda_{\min}(A) - \epsilon)}.$$

Now, note that $\lambda_{\min}(A) - \epsilon \geq \lambda_{\min}(A)/2$, which concludes the proof. □

**Lemma A.2.** *Let* $A = (a_{ij})$ *and* $B = (b_{ij})$ *be symmetric* $2 \times 2$ *matrices. If* $A$ *is positive definite with* $a_{11}, a_{22} \geq \alpha$ *for some constant* $\alpha > 0$ *and* $||A - B||_\infty \leq \epsilon \leq \alpha/2$*, then*

$$\left| \frac{a_{12}}{\sqrt{a_{11}a_{22}}} - \frac{b_{12}}{\sqrt{b_{11}b_{22}}} \right| \leq \frac{4\epsilon}{\alpha}.$$

*Proof.* Let $A' = \frac{1}{\alpha}A$ and $B' = \frac{1}{\alpha}B$. Therefore, we have $||A' - B'||_\infty \leq \epsilon/\alpha \leq 1/2 < 1$. From Lemma 7 of Harris and Drton [2013], we find that

$$\left| \frac{a_{12}}{\sqrt{(a_{11})(a_{22})}} - \frac{b_{12}}{\sqrt{(b_{11})(b_{22})}} \right| = \left| \frac{a_{12}/\alpha}{\sqrt{(a_{11}/\alpha)(a_{22}/\alpha)}} - \frac{b_{12}/\alpha}{\sqrt{(b_{11}/\alpha)(b_{22}/\alpha)}} \right| \leq \frac{2\epsilon/\alpha}{1 - \epsilon/\alpha} \leq \frac{4\epsilon}{\alpha},$$

where the last inequality follows from the fact that $1 - \epsilon/\alpha > 1/2$. □

**Theorem A.2.** *Assume (A1), (A2), (A3) and (A6). Let* $A_n := \{\text{sign}(\hat{K}_{nO}) = \text{sign}(K^*_{nO})\}$*. Then for any* $\delta \in (0, 1)$*,* $i, j \in \{1, \dots, p_n\}$ *and* $U \subseteq \{1, \dots, p_n\} \setminus \{i, j\}$*, there exists an* $n_0 \in \mathbb{N}$

*such that $n \geq n_0$ entails*

$$\mathbb{P}\left(\left|\hat{\rho}_{nij|U} - \rho^*_{nij|U}\right| > \delta,\ A_n\right) \leq C_2 \exp\left(-C_8 n q_n'^{-6} \delta^2\right),$$

*where $C_2 > 0$ is as in Corollary A.1 and $C_8 > 0$ is a constant depending on $C_3$ from Corollary A.1 and $C_4$, $C_5$ from (A6).*

*Proof.* First, we have from Corollary A.1 that

$$\mathbb{P}(||\hat{K}_{nO} - K^*_{nO}||_2 > \delta,\ A_n) \leq C_2 \exp(-C_3 n q_n'^{-2} \delta^2).$$

Note that $\lambda_{\min}(K^*_{nO}) = \frac{1}{||{K^*_{nO}}^{-1}||_2} \geq \frac{1}{C_4}$, by (A6). For $\delta \in (0,1)$, we apply Lemma A.1 with $A = K^*_{nO}$, $E = \hat{K}_{nO} - K^*_{nO}$ and $\epsilon = \frac{\delta}{2C_4^2} \leq \frac{\delta}{2C_4} < \frac{\lambda_{\min}(K^*_{nO})}{2}$ to obtain that $||\hat{K}_{nO} - K^*_{nO}||_2 \leq \frac{\delta}{2C_4^2}$ implies

$$||\hat{K}_{nO}^{-1} - {K^*_{nO}}^{-1}||_2 \leq \frac{\delta}{C_4^2 \lambda^2_{\min}(K^*_{nO})} \leq \delta.$$

Therefore, we have

$$\mathbb{P}\left(||\hat{K}_{nO}^{-1} - {K^*_{nO}}^{-1}||_2 > \delta,\ A_n\right) \leq C_2 \exp(-C_6 n q_n'^{-2} \delta^2), \tag{2}$$

where $C_6 = C_3/(4C_4^2)$.

Fix $i, j \in \{1, \ldots, p_n\}$ and $U \in \{1, \ldots, p_n\} \setminus \{i, j\}$. Without loss of generality, we assume that the principal submatrices of order 2 and order $(|U| + 2)$ of ${K^*_{nO}}^{-1}$ correspond to $\{X_{ni}, X_{nj}\}$ and $\{X_{nr} : r \in \{i, j\} \cup U\}$ respectively. Recall that $\rho^*_{nij|U}$ and $\hat{\rho}_{nij|U}$ can be written as

$$\rho^*_{nij|U} = -\frac{(\boldsymbol{\Psi}_n^{-1})_{12}}{\sqrt{(\boldsymbol{\Psi}_n^{-1})_{11}(\boldsymbol{\Psi}_n^{-1})_{22}}},\ \textit{and}\ \hat{\rho}_{nij|U} = -\frac{(\hat{\boldsymbol{\Psi}}_n^{-1})_{12}}{\sqrt{(\hat{\boldsymbol{\Psi}}_n^{-1})_{11}(\hat{\boldsymbol{\Psi}}_n^{-1})_{22}}}$$

where $\boldsymbol{\Psi}_n = ({K^*_{nO}}^{-1})_{(i,j,U)}$ and $\hat{\boldsymbol{\Psi}}_n = (\hat{K}^{-1}_{nO})_{(i,j,U)}$ are the concerned principal submatrices of ${K^*_{nO}}^{-1}$ and $\hat{K}^{-1}_{nO}$ respectively. Since $||\hat{\boldsymbol{\Psi}}_n - \boldsymbol{\Psi}_n||_2 \leq ||\hat{K}^{-1}_{nO} - {K^*_{nO}}^{-1}||_2$, from (2), we have

$$\mathbb{P}\left(||\hat{\boldsymbol{\Psi}}_n - \boldsymbol{\Psi}_n||_2 > \delta,\ A_n\right) \leq C_2 \exp(-C_6 n {q'_n}^{-2} \delta^2). \tag{3}$$

In order to obtain an upper bound of $\mathbb{P}\left(||\hat{\boldsymbol{\Psi}}_n^{-1} - \boldsymbol{\Psi}_n^{-1}||_\infty > \delta,\ A_n\right)$, we first note that $\lambda_{\min}(\boldsymbol{\Psi}_n) \geq \lambda_{\min}({K^*_{nO}}^{-1}) = \frac{1}{||K^*_{nO}||_2} \geq \frac{1}{C_5 q'_n}$, where $C_5$ is as in (A6) and the last inequality follows from

$$||K^*_{nO}||_2 \leq \text{degree}(K^*_{nO})||K^*_{nO}||_\infty = q'_n C_5.$$

This inequality was derived in the proof of Corollary A.1.

Next, by applying Lemma A.1 with $A = \boldsymbol{\Psi}_n$, $E = \hat{\boldsymbol{\Psi}}_n - \boldsymbol{\Psi}_n$ and $\epsilon = \frac{\delta}{2C_5^2 {q'_n}^2}$, we obtain that for $\delta \in (0,1)$,

$$\mathbb{P}\left(||\hat{\boldsymbol{\Psi}}_n^{-1} - \boldsymbol{\Psi}_n^{-1}||_2 > \delta,\ A_n\right) \leq C_2 \exp(-C_7 n {q'_n}^{-6} \delta^2),$$

where $C_7 = C_6/(4C_5^2)$. By using the inequality $||A||_\infty \leq ||A||_2$, we obtain

$$\mathbb{P}\left(||\hat{\boldsymbol{\Psi}}_n^{-1} - \boldsymbol{\Psi}_n^{-1}||_\infty > \delta,\ A_n\right) \leq C_2 \exp(-C_7 n {q'_n}^{-6} \delta^2). \tag{4}$$

Finally, we will use Lemma A.2 with $A$ and $B$ equal the principal submatrices of order 2 of $\boldsymbol{\Psi}_n^{-1}$ and $\hat{\boldsymbol{\Psi}}_n^{-1}$ respectively, and with $\alpha = 1/C_4$, where $C_4$ is as in (A6) and $(\boldsymbol{\Psi}_n^{-1})_{11}, (\boldsymbol{\Psi}_n^{-1})_{22} \geq \alpha$ follows from

$$(\boldsymbol{\Psi}_n^{-1})_{ii} \geq \lambda_{\min}(\boldsymbol{\Psi}_n^{-1}) = \frac{1}{||\boldsymbol{\Psi}_n||_2} \geq \frac{1}{||{K^*_{nO}}^{-1}||_2} = \frac{1}{C_4},\ \text{for i=1,2.}$$

Therefore, Lemma A.2 and (4) imply that for $\delta \in (0,1)$,

$$\mathbb{P}\left(\left|\hat{\rho}_{nij|U} - \rho^*_{nij|U}\right| > \delta,\ A_n\right) \leq \mathbb{P}\left(||\hat{\boldsymbol{\Psi}}_n^{-1} - \boldsymbol{\Psi}_n^{-1}||_\infty > \delta/4C_1,\ A_n\right) \leq C_2 \exp(-C_8 n {q'_n}^{-6} \delta^2)$$

where $C_8 = C_7/(16C_4^2)$. □

**Corollary A.2.** *Assume the conditions of Theorem A.2. Let* $h(\rho) := (-0.5\log(1-\rho^2))^{1/2}$ *and* $A_n$ *be as in Theorem A.2. Then for any* $\delta \in (0,1)$, $i,j \in \{1,\ldots,p_n\}$ *and* $U \subseteq \{1,\ldots,p_n\} \setminus \{i,j\}$,

$$\mathbb{P}\left(\left|h(\hat{\rho}_{nij|U} - \rho^*_{nij|U})\right| > \delta,\ A_n\right) \leq 2C_2 \exp\left(-C_9 n q_n'^{-6} \delta^2\right),$$

*where* $C_2 > 0$ *is as in Corollary A.1 and* $C_9 > 0$ *is a constant depending on* $C_3$ *from Corollary A.1,* $M$ *from (A5),* $C_4$ *and* $C_5$ *from (A6) only.*

*Proof.* Our claim follows from Theorem A.2, by the arguments given in Corollary 9.1 of the supplementary materials of Nandy et al. [2017] and Lemma 3 of Kalisch and Bühlmann [2007]. The main idea is to apply the mean value theorem to obtain

$$h(\hat{\rho}_{nij|U}) - h(\rho^*_{nij|U}) = h'(\tilde{\rho}_{nij|U})(\hat{\rho}_{nij|U} - \rho^*_{nij|U}),$$

where $|\tilde{\rho}_{nij|U} - \rho^*_{nij|U}| < |\hat{\rho}_{nij|U} - \rho^*_{nij|U}|$. Then we can obtain upper bounds on $\mathbb{P}(|h'(\tilde{\rho}_{nij|U})| > L,\ A_n)$ and $\mathbb{P}(|\hat{\rho}_{nij|U} - \rho^*_{nij|U}| > \delta/L,\ A_n)$ separately, where $L := 1/(1-(1+M)^2/4)$. □

**Proof of Theorem 3.1.** Let $A_n := \{\text{sign}(\hat{K}_{nO}) = \text{sign}(K^*_{nO})\}$. It suffices to show that $\mathbb{P}(\hat{\mathcal{C}}_{nO} \neq \mathcal{C}^*_{nO},\ A_n) \to 0$, since by assumption (A1), $\mathbb{P}(A_n) \to 1$.

Following Nandy et al. [2017], we choose $\lambda_n = -\frac{1}{9}(1-c_n^2)$, where $c_n$ is given by (A5). We define the set

$$E_{nij|U} := \{\left|h(\hat{\rho}_{nij|U}) - h(\rho^*_{nij|U})\right| > \sqrt{\lambda_n}\} \cup \{|\hat{\rho}_{nij|U} - \rho^*_{nij|U}| > \delta_n/2\},$$

for $i \neq j$ and $U \subseteq \{1,\ldots,p_n\} \setminus \{i,j\}$, where $\delta_n$ is given by assumption (A4), $h(\rho) = (-0.5\log(1-\rho^2))^{1/2}$. We further define

$$\mathbf{U}_{i,j}^{K_n q_n} := \{U \subseteq \{1,\ldots,p_n\} \setminus \{i,j\} : |U| \leq K_n q_n\}.$$

By the arguments given in the proof of Theorem 5.2 of Nandy et al. [2017], it follows that

$$\mathbb{P}(\hat{\mathcal{C}}_{nO} \neq \mathcal{C}^*_{nO},\ A_n) \leq \mathcal{O}(p_n^{K_n q_n + 2}) \sup_{i,j,U \in \mathbf{U}_{i,j}^{K_n q_n}} \mathbb{P}(E_{nij|U} \cap A_n).$$

Without loss of generality, we assume that $\lambda_n, \delta_n < 1$ for all $n$. Then by Theorem A.2 and Corollary A.2 above, we have

$$\sup_{i,j,U \in \mathbf{U}_{i,j}^{K_n q_n}} \mathbb{P}(E_{nij|U} \cap A_n) \leq \mathcal{O}\left(\exp\left(-C' q_n'^{-6} n \min(\lambda_n, \delta_n^2)\right)\right),$$

for some constant $C' > 0$. Note that $\lambda_n = -\frac{1}{9}\log(1 - c_n^2) \sim c_n^2/9$ as $c_n \to 0$, and by assumptions (A4) and (A5), $c_n^{-2} = \mathcal{O}(n^{2d_2})$ and $\delta_n^{-2} = \mathcal{O}(n^{2d_1})$. Therefore, for sufficiently large $n$,

$$\mathbb{P}(\hat{\mathcal{C}}_{nO} \neq \mathcal{C}^*_{nO},\ A_n) \leq \mathcal{O}\left(\exp((K_n q_n + 2)\log(p_n) - C'' q_n'^{-6} n^{1-2\max(d_1,d_2)})\right),$$

for some constant $C'' > 0$. This completes the proof, since $(K_n q_n + 2)\log(p_n) = \mathcal{O}(n^{1-f}\log(n))$ and $2\max(d_1, d_2) < f$ (by assumptions (A4) and (A5)).

# B Additional Simulation Results

We complement the results of Section 4.1 by reporting the performances of the various methods for the recovery of directed edges. We considered two sets of directed edges:

i) We first compared the directed edges of the estimated CPDAGs to the directed edges of the true CPDAG. For the NSDIST method, which returns a DAG and not a CPDAG, we used the R function `dag2cpdag` of the `pcalg` package. In any case, undirected edges are ignored.

ii) We also compared the estimated graphs to the true DAG. For methods that return a CPDAG, we treated the undirected edges as 1/2 false negative and 1/2 false positive, as in Han et al. [2016]. NSDIST, which returns a DAG, was compared directly to the true DAG.

Figure 1 shows the precision vs. recall curves in terms of directed edges recovery (set i)), for both simulation designs. In Figure 1 **a)**, we see that LRpS+GES is outperformed by PCA+GES and PEER+GES when the sample size is small ($n = 50$). This is in contrast with Figure 2 **a)** of the main paper, where LRPS+GES was outperforming other methods in terms of *skeleton* recovery. We believe that this is due to the tuning parameters of LRpS being chosen with cross-validation. Here, the number of samples $n$ and the dimension of the problem ($p$) are identical, but the expected number of edges is greater than $n$ (about 60). This often results in values of $\gamma$ that are too small. In contrast, we recall that for PEER*+GES and PCA*+GES the number of latent components is chosen so as to maximise the area under the precision/recall curve for skeleton recovery. We found that when using a similar strategy to select the tuning parameters of LRpS ($\eta_n, \gamma$), it performed at least as well the other methods when $n = 50$.

Figure 2 shows the precision vs. recall curves in terms of DAG recovery (set ii)), for both simulation designs. Results are similar to those shown in Figure 1, but NSDIST performs comparatively better.

Finally, in Figure 3 we report the distribution of incoherences for the latent component $L^*$ in our second simulation design. Figure 3 **a)** shows that the set of models we draw from is rather challenging, with the bulk of $inc(L^*)'s$ distribution located close to 1. Figure 3 **b)** shows the impact of the number of latent components $h$ on $inc(L^*)$. While a large value of $h$ strongly correlates with high values of $inc(L^*)$, this plot shows that there instances in which $inc(L^*)$ is high and $h$ is small. These correspond to cases where the hidden variables

a)

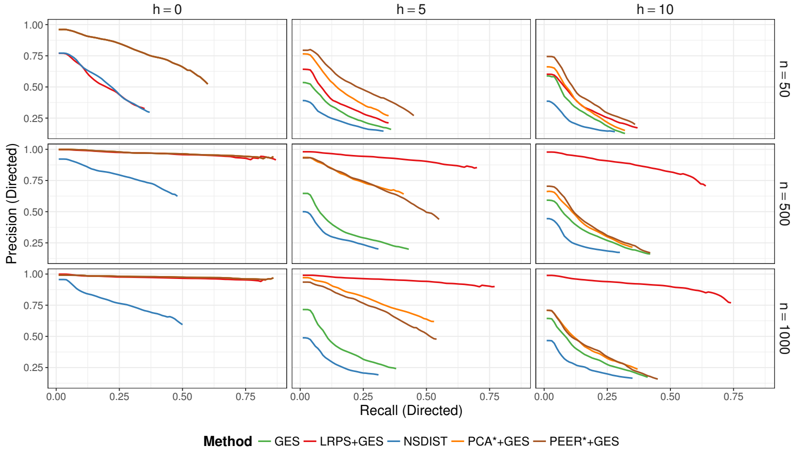


b)

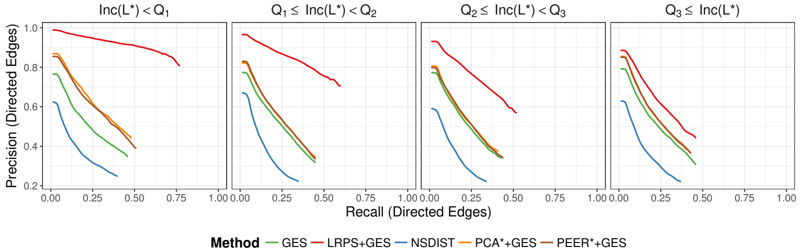


Figure 1: Average precisions at fixed recalls of $\{0.01, 0.02, \ldots, 1\}$ for the recovery of the CPDAG's directed edges (set i)). There are $p = 50$ observed variables. **a)** Effect of the number of hidden variables ($h$) and sample size ($n$), when $f = 70$ and each of the 9 designs is repeated 50 times. **b)** Effect of the incoherence of the latent structure $inc(L^*)$. The 500 random datasets are binned according to the quartiles of $inc(L^*)$'s distribution ($Q_1 - Q_4$).

act on the observed ones in a sparse fashion.

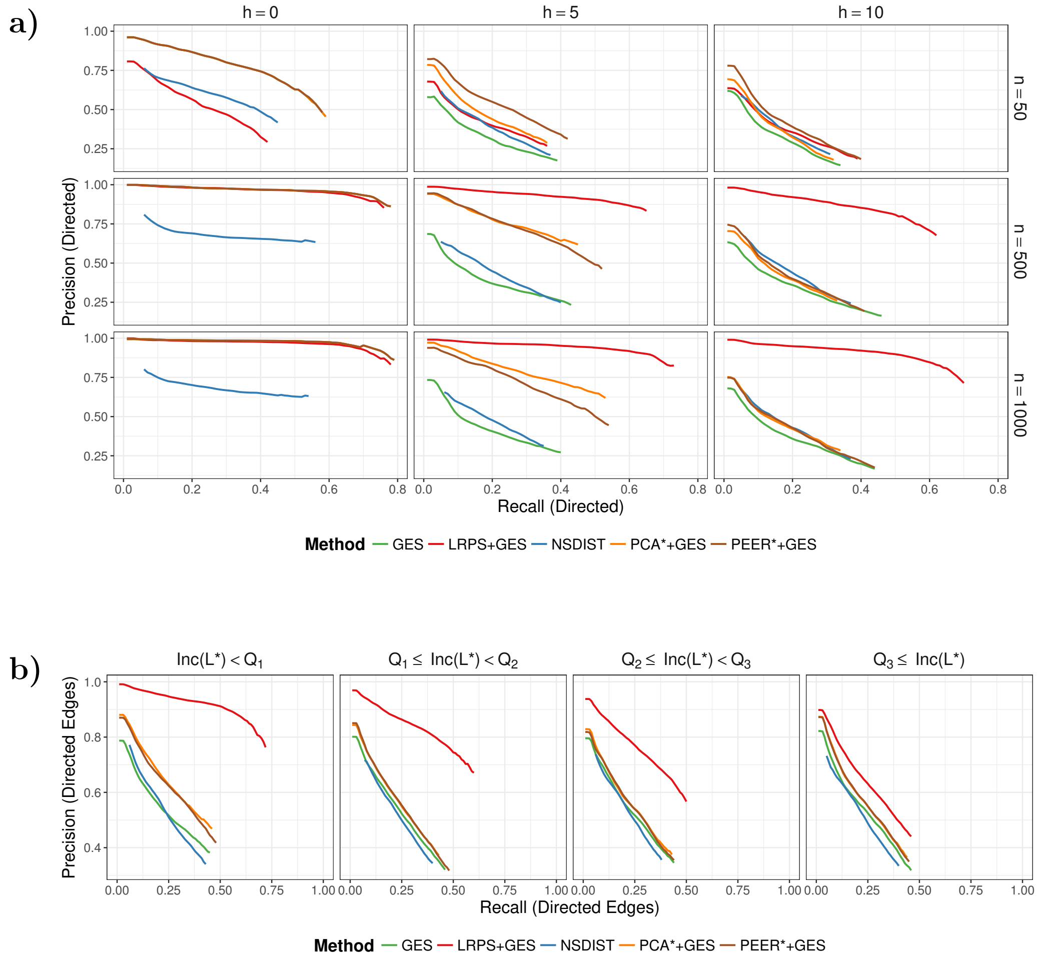


Figure 2: Precision vs. recall curves for DAG recovery (set ii)). There are $p = 50$ observed variables. We report average precisions at fixed recalls of $\{0.01, 0.02, \ldots, 1\}$. **a)** Effect of the number of hidden variables ($h$) and sample size ($n$) when $f = 70$ and each of the 9 designs is repeated 50 times. **b)** Effect of the incoherence of the latent structure $inc(L^*)$. The 500 random datasets are binned according to the quartiles of $inc(L^*)$'s distribution ($Q_1 - Q_4$).

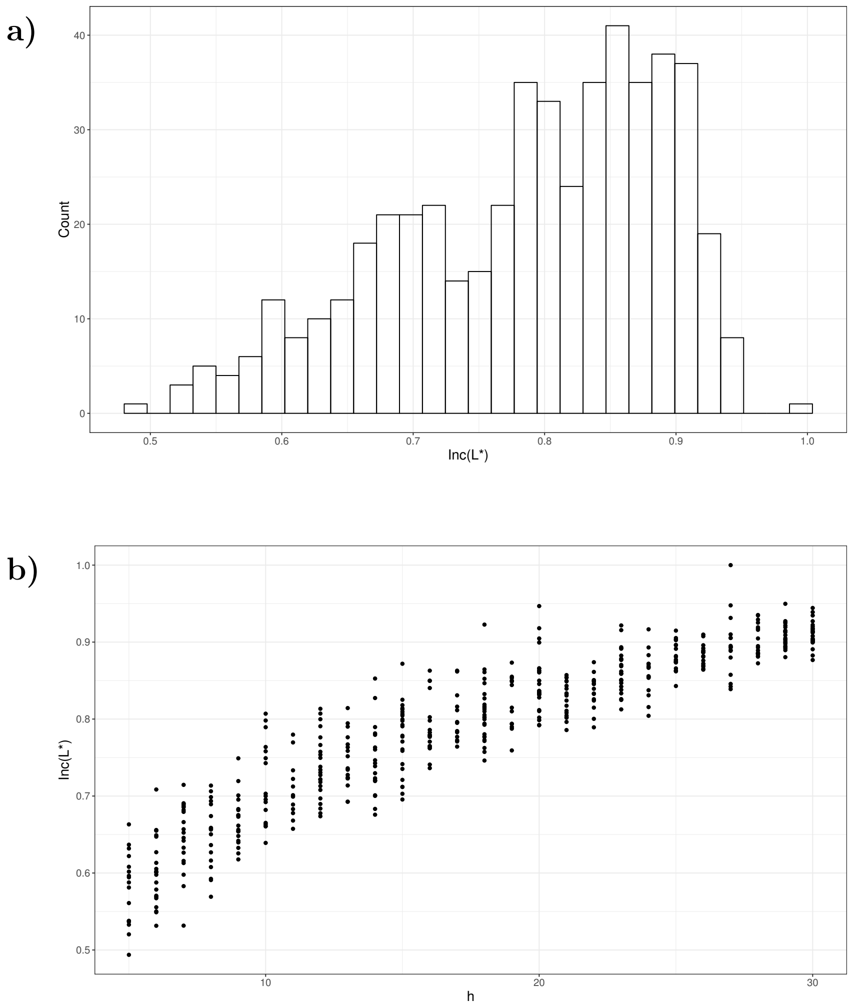


Figure 3: **a)** Distribution of $inc(L^*)$ in the second simulation setting described in Section 4.1. **b)** Effect of the number of hidden variables ($h$) on $inc(L^*)$.

# C Additional Results for Application 1

We report results in terms of DAG estimation and total causal effect estimation for the methods that have been left out of Section 5.1: PEER+GES, PCA+GES and NSDIST. These methods are described in our simulations (§4.1). For each of these methods, a graph is chosen along their respective regularisation path using the BIC.

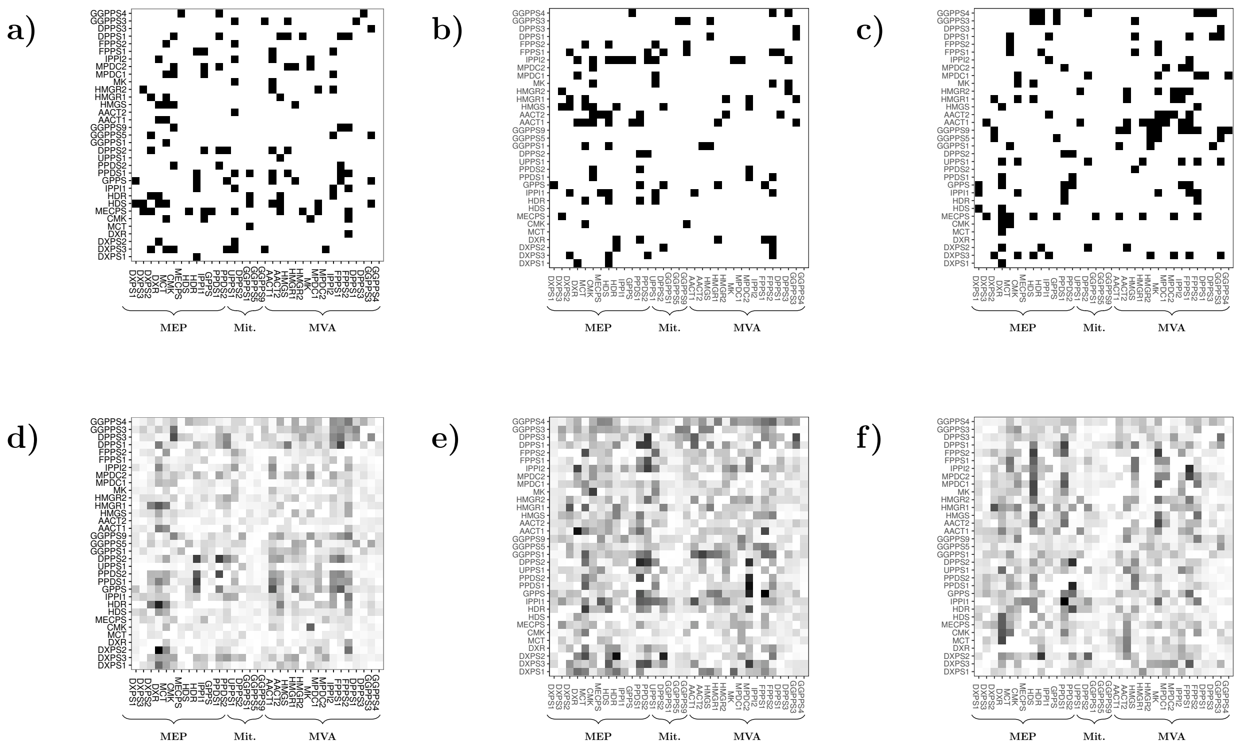


Figure 4: Estimates obtained by applying PEER+GES, PCA+GES and NSDIST to the data of Wille et al. [2004]. **a)** Adjacency matrix of the CPDAG estimated by PEER+GES. **b)** As in a), but with PCA+GES. **c)** DAG estimated by NSDIST. **d)** Matrix of total causal effects for (PEER+GES),IDA. **e)** As in d), but with PCA+GES. **f)** Matrix of total causal effects for NSDIST,IDA.

# References

Chandrasekaran, V., Parrilo, P. A. and Willsky, A. S. [2012], 'Latent variable graphical model selection via convex optimization', *Ann. Statist.* **40**, 1935–1967.

Han, S. W., Chen, G., Cheon, M.-S. and Zhong, H. [2016], 'Estimation of directed acyclic graphs through two-stage adaptive lasso for gene network inference', *J. Am. Statist. Ass.* **111**, 1004–1019.

Harris, N. and Drton, M. [2013], 'PC algorithm for nonparanormal graphical models', *J. Mach. Learn. Res.* **14**, 3365–3383.

Kalisch, M. and Bühlmann, P. [2007], 'Estimating high-dimensional directed acyclic graphs with the PC-algorithm', *J. Mach. Learn. Res.* **8**, 613–636.

Nandy, P., Hauser, A. and Maathuis, M. H. [2017], High-dimensional consistency in score-based and hybrid structure learning. Available at: arXiv:1507.02608.

Wille, A., Zimmermann, P., Vranová, E., Fürholz, A., Laule, O., Bleuler, S., Hennig, L., Prelić, A., von Rohr, P., Thiele, L., Zitzler, E., Gruissem, W. and Bühlmann, P. [2004], 'Sparse graphical Gaussian modeling of the isoprenoid gene network in arabidopsis thaliana', *Genome Biology* **5**(11), R92.
